# Supplementary material for: Accessing the strong interaction between $\Lambda$ baryons and charged kaons with the femtoscopy technique at the LHC
Source: arXiv:2305.19093 source file (2023-10-11)
Supplement: Supplementary file 1 [file Appendix.tex]

\section{Additional material}
